# Supplementary material for: Graph theory-based structural analysis on density anomaly of silica glass
Source: arXiv:2111.07452 source file (2022-08-23)
Supplement: Supplementary file 1 [file SupportingInformation.pdf]

Supporting Information for

# Graph theory-based structural analysis on density anomaly of silica glass

Aik Rui Tan,[1, §] Shingo Urata,[*,2, §,†] Masatsugu Yamada,[3] and Rafael Gómez-Bombarelli[*,1,‡]

[1]Department of Materials Science and Engineering, Massachusetts Institute of Technology

[2]Technology General Division, Planning Division, AGC Inc.

[3]Innovative Technology Laboratories, AGC Inc.

[§] Both authors contributed equally

[†] shingo.urata@agc.com

[‡] rafagb@.mit.edu

*Corresponding authors

**Table S1**. Fictive temperature determined from potential-temperature curve. Average, μ and standard deviation, σ were evaluated using five independent replicas of glass-v1 and glass-v2 generated from FMP-v1 and FMP-v2, respectively.

| | **Glass-v1** | | | | | **Glass-v2** |
|---|---|---|---|---|---|---|
| | a-$SiO_2$ | $SiO_2$-F1 | $SiO_2$-F3 | $SiO_2$-F5 | $SiO_2$-F10 | a-$SiO_2$ |
| μ (K) | 1899 | 1933 | 1848 | 1802 | 1586 | 2540 |
| σ (K) | 18 | 13 | 17 | 80 | 43 | 11 |

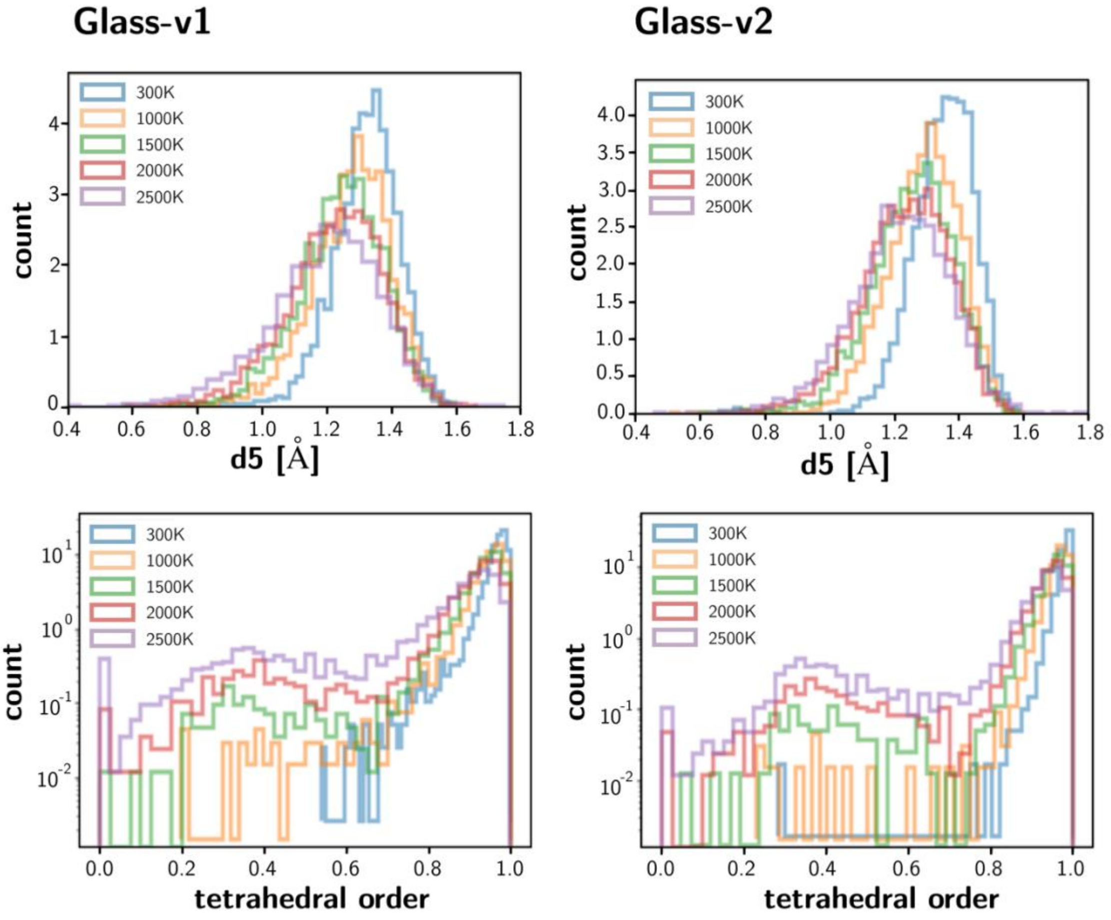


**Figure S1**. Histograms showing comparison between glass-v1 and glass-v2 of (Upper) d5, which represents distance between 4th neighbor oxygen and the nearest silicon from a central silicon and (Lower) tetrahedral order of $SiO_4$ units defined as,

$$q = 1 - \frac{3}{8}\sum_{i=1}^{3}\sum_{j=i+1}^{4}\left(cos\phi_{ij} + \frac{1}{3}\right)^{3}$$

where $f_{ij}$ is the angle between two vectors from the central silicon to two of the nearest oxygen.
